# Supplementary material for: Only distances are required to reconstruct submanifolds
Source: arXiv:1410.7012 source file (2017-08-05)
Supplement: Supplementary file 2 [file appendix-power-protection.tex]

\subsection{Proof of Lemma~\ref{lem:dim-voronoi-protected-simplex}}
\label{appendix-power-protection}

For the rest of this section we will assume the following hypothesis:

\begin{hyp}
    Let $\pts \subset \R^{d}$ be a finite point sample, and let
    $\omega: \pts \rightarrow [0, \infty)$ be a weight assignment such that
    there exists $p \in \pts$ with $\vor_{\omega}(p)$ is bounded.
\end{hyp}
Since $\vor_{\omega}(p)$ is bounded, we have $\dim \aff (\pts) = d$.

The following lemma is analogous to~\cite[Lem.~3.2]{boissonnat2012sdt}, and 
the proof is exactly samce as that lemma.

\begin{lem}[Maximal simplices]\label{lem-maximal-simplices-incident-p}
    Every $\sigma \in \del_{\omega}(\pts)$ incident to $p$
    is a face of a simplex $\sigma' \in \del_{\omega}(\pts)$ 
    with $\dim\aff(\sigma')= d$.
\end{lem}
Following lemma is a direct consequence is the above result.
\begin{lem}[No degeneracies]\label{lem-no-degeneracies-incident-p}
    If every $d$-simplex in $\del_{\omega}(\pts)$ incident to $p$
    is
    $\delta^{2}$-power protected for some $\delta > 0$, then there are no
    degenerate simplices in $\del_{\omega}(\pts)$ incident to $p$.
\end{lem}

Like in the case of Lemma~\ref{lem-maximal-simplices-incident-p}, 
following result is analogous to~\cite[Lem.~3.3]{boissonnat2012sdt}
and can be proved exactly along the same lines.
\begin{lem}[Separation]\label{lem-separation-result}
  If $\sigma^{j} \in \del_{\omega}(\pts)$ is a $j$-simplex incident to $p$, 
  and $q \in \pts \setminus \sigma^{j}$, then there is a $d$-simplex 
  $\sigma^{d} \in \del_{\omega}(\pts)$ incident to $p$ such that 
  $\sigma^{j} \leq \sigma^{d}$ and $q \not\in \sigma^{d}$.
\end{lem}

We will need the definition of $N_{\omega}(\sigma)$ defined in 
Section~\ref{sec-appendix-notations}.

\begin{proof}[of Lemma~\ref{lem:dim-voronoi-protected-simplex}]
  Let $\sigma^{k} \in \del_{\omega}(\pts)$ 
  be a maximal $k$-simplex
  incident to $p$ such that 
  $\dim \vor_{\omega}(\sigma^{k}) < d - k$. From 
  Lemma~\ref{lem-no-degeneracies-incident-p}, we have $k < d$.
  We can generate, from Lemma~\ref{lem-maximal-simplices-incident-p}, 
  a sequence of simplices
  $$
    \sigma^{k} < \sigma^{k+1} < \dots < \sigma^{d}
  $$
  where $\sigma^{j} \in \del_{\omega}(\pts)$ and 
  $j \in \{k,\, \dots, \, d \}$. 

  Let $q = \sigma^{k+1} \setminus \sigma^{k}$. From
  Lemma~\ref{lem-separation-result}, there exists 
  a $d$-simplex $\sigma \in \del_{\omega}(\pts)$ such that 
  $\sigma^{k} < \sigma$ and $q \not\in \sigma$. Let 
  $c \in \vor_{\omega}(\sigma)$. Since the $d$-simplices 
  incident to $p$ is $\delta^{2}$-power protected, 
  it is easy to see that $\exists~ \delta' > 0$ such that
  $\forall~x \in B(c,\delta')$, we have
  \begin{equation}
    d(x, q^{\omega}) < d(x, r^{\omega}),
    ~\forall~ q \in \sigma ~\mbox{and}~ r \in \pts \setminus \sigma 
  \end{equation}
  This implies 
  $N_{\omega}(\sigma^{k})\cap B(c,\delta') \subseteq \vor_{\omega}(\sigma^{k})$,
  and since $c \in N_{\omega}(\sigma^{k})$, we get a contradiction 
  with the initial assumption that 
  $\dim \vor_{\omega}(\sigma^{k}) < d - k$.
\end{proof}
